# Supplementary material for: Tricks for Training Sparse Translation Models
Source: arXiv:2110.08246 source file (2021-10-15)
Supplement: Supplementary file 1 [file appendix.tex]

\section{Appendices}

% \subsection{Expert distribution for temperature heating}

% WMT-15
\begin{table*}[!t]
\centering
    \small
    \begin{tabular}{lcccccccc}
    \toprule
     Language & \multicolumn{2}{c}{\textbf{Baselines}} & \multicolumn{5}{c} {\textbf{starting temperature ($t_s$)}} \\
    \cmidrule(lr){2-3}  \cmidrule(lr){4-8}  
     &   {Dense} & {BASELayers}  & {0.5} & {0.8} &  {1}  & {1.5} & {2} \\
     \midrule
      \textcolor{teal}{\textbf{cs}} & 21.5 & 21.4  & 22.5 & 22.3 & 22.2 & 21.9 & 21.7 \\
      \textcolor{teal}{\textbf{de}} & 23.9 & 24 & 24 & 24.7 & 24.2 & 24.5 &  24.3 \\ 
      \textcolor{teal}{\textbf{es}} & 30 & 29.8  & 30.6 & 30.9 & 30.3 & 29.7 & 29.7 \\
      \textcolor{teal}{\textbf{et}} & 19 & 18.8  & 18.4 & 19.3 & 18.5 & 19.4 & 18.8 \\
      \textcolor{teal}{\textbf{fi}} & 19.6 & 19.5  & 19.9 & 20.6 & 19.9 & 20.2 & 20.0 \\
     \textcolor{teal}{\textbf{fr}} & 33.2 & 32.5  & 34.2 & 34.4 & 35.3 & 34.9 & 33.1 \\
     \textcolor{teal}{\textbf{ru}} & 27 & 27.6 & 28.3 & 28.6 & 28.6 & 28.1 & 26.8 \\
     \textcolor{teal}{\textbf{zh}} & 29.2 & 29 & 30.2 & 30.1 & 20 & 29.7 & 29.2 \\
     \textcolor{magenta}{\textbf{gu}} & 9.7 & 8.2  & 9.2 & 8.7 & 9.5 & 9.5 & 9.2\\
      \textcolor{magenta}{\textbf{hi}} & 12.9 & 11.7 & 12.9 & 13.4 & 13.2 & 12.6 & 12.8   \\
      \textcolor{magenta}{\textbf{kk}} & 4.2 & 3.8  & 4.4 & 3.7 & 4.3 & 4.5 & 4.3\\
      \textcolor{magenta}{\textbf{lt}} & 13 & 12.4  & 12.4 & 12.7 & 12.8 & 12.3 & 13.1  \\
      \textcolor{magenta}{\textbf{lv}} & 16.2 & 15.7 & 15.8 & 15.9 & 15.1 & 15.6 & 15.9 \\
      \textcolor{magenta}{\textbf{ro}} & 25 & 25 & 25.2 & 25 & 24.9 & 25 & 25.2\\
      \textcolor{magenta}{\textbf{tr}} & 12 & 11.8  & 12 & 11.9 & 12.2 & 12.1 & 12.5 \\
      \midrule 
      \textbf{Average} & 19.76 & 19.41 & 20 & 20.09 & 20.08 & 20 & 19.77 \\
      \textbf{Avg. Low Res.} & 13.28 & 12.65 & 13.13 & 12.93 & 13.17 & 13.09 & 13.28 \\
      \textbf{Avg. High Res.} & 25.43 & 25.32 & 26.01 & 26.36 & 26.13 & 26.05 & 25.45 \\
      \textbf{Wall (min)} & 89K  & 61K & 189K & 179K & 123K & 80K & 76K \\
    %   \textbf{Wall (min)} & 89140  & 61149 & 189449 & 179557 & 123848 & 80004 & 76281 \\
    \bottomrule
    \end{tabular}
    \caption{\textbf{WMT-15} --- Average and task-specific BLEU and wall clock training time (until convergence) for different starting temperatures across 8 \textcolor{teal}{\textbf{high resource}} and 7 \textcolor{magenta}{\textbf{low resource}} languages with a fixed conduction rate, $k$=1. The baselines are from our best performing dense and BASELayers model trained with fixed temperature of 2.}
    \label{tab:temp_samp_wmt15_full}
\end{table*}

\begin{table*}[htp]
\centering
    \small
    \begin{tabular}{lcccc}
    \toprule
     \textbf{Model} & \textcolor{teal}{High Resource} & \textcolor{magenta}{Low Resource} & All & Wall (min)\\
     \midrule
        % \textbf{Dense, tmp=2} & 25.42 & 13.28 & 19.76 & 89410  \\
        Dense & 25.15 & 12.74 & 19.36 & 76049  \\
        +heating & 25.5 & 13.18 & 19.76 & 42133  \\
        BASELayers & 25.2 & 12.9 & 19.46 & 77561 \\
        +heating & 26.0 & 13.0 & 19.91 & 42154  \\
     \midrule
       30k & 25.71 & 13.14 & 19.85 & 58951 \\
        +heating & 24.68 & 13.31 & 19.38 & 54845 \\
       40k & 25.82 & 13.11 & 19.90 & 50819 \\
        +heating & 25.85 & 13.24 & 19.97 & 43964 \\
        50k & 26.10 & 13.34 & 20.13 & 100503   \\
        +heating & 25.78 & 13.18 & 19.91 & 40719 \\
        60k & 26.30 & 13.28 & \textbf{20.21} & 86944  \\
        +heating & 25.98 & 13.43 & \textbf{20.13}  & 31459 \\
        70k & 25.8 & 13.25 & 19.95 & 80071 \\
        +heating & 25.98 & 13.47 & 20.15 & 35792 \\
       80k & 25.79 & 13.16 & 19.90 & 50751\\
        +heating & 26.05 & 13.33 & 20.11 & 35680  \\
        90k &  25.66 & 13.15 & 19.83 & 54452\\
        +heating & 25.93 & 13.41 & 20.10 & 40744  \\
    \bottomrule
    \end{tabular}
    \caption{\textbf{WMT-15} --- Average test set BLEU with increasing number of dense pre-training steps at a starting/fixed temperature of 1.5. Wall clock time is the total training time including dense pre-training and MoE fine-tuning until the model reach 5.99 validation ppl.}
    \label{tab:pretrain_results_wmt15_full}
\end{table*}

\begin{table*}[htp]
\centering
    \small
    \begin{tabular}{lcccccc}
    \toprule
     Model & \textcolor{teal}{\textbf{High Resource}} & \textcolor{brown}{\textbf{Mid Resource}}  & \textcolor{magenta}{\textbf{Low Resource}} & \textbf{All} & \textbf{Wall (min)} \\
     \midrule
     Dense  & 24.7 & 23.65 & 10.71 & 22.5  & 596K  \\ %596164
     +heating & 25.9 & 23.39 & 10.46 & 22.7 & 173K \\ %173730
     BASELayers & 26.6  & 22.56  & 8.74 & 22.2  & 221K \\ %221358
     +heating &  26.5 & 23.04 & 9.1 & 22.53 & 151K \\ %151358
     \midrule
      Epoch=2 & 26.96 & 22.75 & 9.48 & 22.52 & 126K \\ %126978
      +heating & 26.88 & 22.89 & 9.62   & 22.6 &  90K \\ %90292
      Epoch=3 & & & & & 122K \\ %122668
      +heating  & 26.73 & 23.03 & 9.82 & 22.7 & 87K \\ %87412
      Epoch=4 & 26.98 & 22.94 & 9.58 & 22.65 & 106K \\ %106244
      +heating & 26.61 & 23  & 9.68 & 22.6  &  94K  \\ %94144
      Epoch=5 & & & & &  147K  \\ %147688
      +heating &  26.57 &  23 & 9.88 & 22.6 & 115K \\ %115997
    \bottomrule
    \end{tabular}
    \caption{\textbf{ML-50} --- Average test set BLEU, with increasing number of dense pre-training steps with $t_s$=1.5, $k$=2. Wall clock time is the total training time including dense pre-training and MoE fine-tuning until the model reached validation ppl 7.6. The baseline dense results are the best performing results from original paper.}
    \label{tab:pretrain_results_ml50}
\end{table*}
